# Supplementary material for: VEIL: Vetting Extracted Image Labels from In-the-Wild Captions for Weakly-Supervised Object Detection
Source: arXiv:2303.09608 source file (2024-03-10)
Supplement: Supplementary file 1 [file data_appendix.tex]

\section{Caption Label Noise Data Appendix}
This section will provide details on how the dataset was created as well as more details on annotator agreement. We use three in-the-wild datasets to construct this dataset. We perform weighted sampling, the same weighted sampling applied to WSOD, and draw 100 VAELs, their caption, and corresponding image from each in-the-wild VL dataset. 
\begin{figure}
    \centering
    \includegraphics{iccv2023AuthorKit/figures/images/vael_cat_distribution.png}
    \caption{CLaN VAEL Category Distribution}
    \label{fig:vael_cat_distribution}
\end{figure}
\subsection{Annotation Interface}
\begin{figure}
    \centering
    \includegraphics{iccv2023AuthorKit/figures/images/annot_interface.png}
    \caption{Annotation Interface}
    \label{fig:annot_interface}
\end{figure}

After annotating 100 examples from RedCaps, the two annotators calibrated their responses based on disagreement and aligning their subjectivity. We find that agreement goes up for each question after this. RedCaps was not re-annotated.

\subsection{Agreement}
\begin{figure}
    \centering
    \includegraphics{iccv2023AuthorKit/figures/images/agreement_by_option_sbucaps.png}
    \includegraphics{iccv2023AuthorKit/figures/images/agreement_by_option_redcaps.png}
    \includegraphics{iccv2023AuthorKit/figures/images/agreement_by_option_cc.png}
    \caption{Agreement by Option for Q4}
    \label{fig:agreement_by_option}
\end{figure}
