# Supplementary material for: VEIL: Vetting Extracted Image Labels from In-the-Wild Captions for Weakly-Supervised Object Detection
Source: arXiv:2303.09608 source file (2024-03-10)
Supplement: Supplementary file 2 [file supp_dump.tex]

\section{Case Study: Additional Analysis on Descriptiveness/Narrativeness}

\subsection{Linguistic Differences}
Table \ref{tab:pos_dii_sis} presents the distribution of part-of-speech tags in DII and SIS captions, revealing a significant disparity in frequency across various parts of speech. We show that verb tense is more evenly distributed in narrative than descriptive captions which favor present tense. Additionally, Table \ref{tab:aspect} shows aspect, inferred using part-of-speech tags. Aspect relates to visual-text alignment. Progressive aspect refers to verbs that describe an ongoing, hence likely to be shown, activity such as ``The event is starting, there are even some dancers forming outside" while perfective describes a completed or close to completion activity, e.g. ``The old part has been \textbf{removed} and now there many loose wires now". Table \ref{tab:aspect} shows that progressive aspect is more common in both, but very frequent in DII captions, which aligns with our expectations. 
\begin{table}[!htb]
      \centering
        \begin{tabular}{|r|c|c|}\hline
            Part of Speech   & DII & SIS \\ \hline
            noun   & \textbf{3.85} & 2.73 \\
            preposition  & \textbf{1.75} & 1.01 \\
            adjective   & \textbf{0.98} & 0.85 \\
            personal pronoun   & 0.18 & \textbf{0.80} \\\hline
            \textbf{verb}   &1.55 & \textbf{2.00}\\\hline
            verb base   & 0.07 & \textbf{0.37}\\
            verb gerund  & \textbf{0.61} & 0.23\\
            past tense  & 0.08 & \textbf{0.89}\\
            past participle  &  \textbf{0.21} & 0.17\\
            non-3rd person sing pres  &\textbf{ 0.22}& 0.16\\
            3rd person sing pres  & \textbf{0.36}& 0.19\\
            \hline
        \end{tabular}
    \caption{The difference in part of speech between descriptive and narrative captions. }
    \label{tab:pos_dii_sis}
\end{table}

\begin{table}
  \centering
    %\caption{Using a random sample of 10,000 captions, we observe verb tense and grammatical aspect. The SIS corpora consists of a slightly imbalanced mix of verbs in the past tense form and present tense form, whereas DII is mainly written in the present form. In terms of aspect, both DII and SIS favor progressive aspect where verbs describe ongoing events rather than completed events.}
    \label{tab:verb_tense_distribution}
    \begin{tabular}{|r|c|r|c|c|}\hline
         & past & present  & progressive & perfective \\ \hline
        DII & 18.5\% & \textbf{81.4\%} &  \textbf{94.5\%} & 5.4\%\\
        SIS & \textbf{52.8\%} & 47.2\% &  \textbf{75.1\%} & 24.9\%\\
        \hline
    \end{tabular}
    \caption{Distribution over tense and aspect. }
    \label{tab:aspect}
\end{table}

\begin{table}[t]
    \centering
    \scalebox{0.95}{
    \begin{tabular}{|r|c|c|}\hline
        Linguistic features & PREC & REC \\\hline
        POS & \textbf{0.8823} & \textbf{0.8782}\\
        CLIP \cite{Radford2021LearningTV} & 0.7215 & 0.7170 \\\hline
        CLIP+POS & 0.8925 & 0.8893\\
        BERT & \textbf{0.9570} & \textbf{0.9560}
        \\\hline % prec dropped from 0.968 -> 0.957 (previously evaluated on a subset)
    \end{tabular}}
    \caption{We evaluate precision/recall of DII/SIS classifiers on a VIST holdout.}
    %taking in combinations of linguistic features 
    %We see that part of speech tags are quite discriminative, however using all features: RST, CLIP*, and CLUE increase the precision and recall of the classifier. 
    %\cite{Radford2021LearningTV}. 
    \label{tab:dii_sis_classifier}
\end{table}

\begin{table*}[t]
    \centering
    \scalebox{0.9}{
    \begin{tabular}{|c|c|c|c|}    \hline
         & DII (Highest scoring) & Random & SIS (Lowest scoring) \\\hline
        Ground Truth Labels & \textbf{0.0195} & 0.0105 & 0.0050\\\hline
        POS-based Classifier &\textbf{0.0304} & 0.0105 & 0.0047\\\hline
        CLIP-based Classifier & \textbf{0.0173} & 0.0105 & 0.0043 \\\hline
    \end{tabular}}
    \caption{mAP when evaluating on VOC-07. Random is independent of the classifier descriptive-ness scores, hence is trained only once.}
    \label{tab:eval_dii_sis_predictions}
\end{table*}

\subsection{Descriptiveness Classifier}
\textbf{Training details.} We examine using part-of-speech tags to discriminate between descriptive and narrative captions, and compare against methods trained with much more data, BERT \cite{BERT} and CLIP \cite{Radford2021LearningTV}. To set up this task, we use captions from the VIST dataset \cite{huang2016visual} which contains multiple captions written in three distinct styles for each image. We use the descriptive-in-isolation (DII) and story-in-sequence (SIS) captions from VIST \cite{huang2016visual} and assign a positive label (descriptive) to captions drawn from the DII split and a negative label (narrative) to captions drawn from the SIS split. We then train a logistic regression model, which we refer to as the descriptiveness classifier. This classifier takes a binary vector corresponding to the presence of a linguistic feature (e.g. proper noun, adjective, verb - past tense, etc) in the caption. The CLIP-based descriptiveness classifier uses only the cosine similarity between the image embeddings and caption embeddings to distinguish between descriptiveness and narrativeness; training a logistic regression model on a single feature has the effect of finding an appropriate threshold for this task. For the BERT upper bound comparison, we finetune BERT without freezing weights.
For this experiment, we sample a balanced subset of VIST with captions containing an exact match with a category from the following constrained label set: dog, boat, person, car. 
We compare different combinations of the input in Table \ref{tab:dii_sis_classifier}.
We find that simple linguistic features such as part-of-speech do nearly as well as BERT \cite{BERT}, despite being much smaller and having less overhead (no forward pass required). Further, POS is stronger than CLIP, and combining them achieves a better results than either one in combination, indicating these features carry complementary information for this task.

\textbf{WSOD applicability.} For this experiment, we sample a balanced subset of VIST with captions containing an exact match with a category from the following constrained label set: dog, boat, person, car. 
Table \ref{tab:eval_dii_sis_predictions} shows that these classifiers can be used to select quality data for training weakly-supervised object detection models. Each classifier assigns descriptiveness scores; we show that when the highest-scoring caption is selected per image (resulting in a pool of descriptive captions), the results are \textbf{4-6 times better} than when selecting the lowest-scoring captions (resulting in narrative captions). Specifically, we extract labels from the selected captions as pseudo image-level labels using exact string matching, to train the multiple instance detection network using WSDDN \cite{bilen2016weakly}. We measure mAP at $IOU=0.5$ over the selected categories (car, boat, dog, person). 

\textbf{Evaluating the descriptiveness classifier on in-the-wild datasets.}
Seeing the low performance of the descriptiveness classifier in vetting of extracted labels (Table 2 in the main text), we hypothesize that this is due to inability of this classifier to distinguish between descriptive/narrative captions in in-the-wild datasets. We thus test the ability of the part-of-speech based descriptiveness classifier trained on VIST descriptive and narrative captions to predict whether an in-the-wild caption is descriptive. As described in the main text, we label 100 captions as having a descriptive or narrative style from SBUCaps, RedCaps and Conceptual Captions. We use the part-of-speech based classifier trained on VIST to predict whether the annotated captions are descriptive; predictions over the threshold 0.5 are classified as descriptive. We use metrics like accuracy, descriptive misclassification rate ($\frac{\text{\# of incorrect descriptive predictions}}{\text{\# of descriptive captions}}$), and narrative misclassification rate ($\frac{\text{\# of incorrect narrative predictions}}{\text{\# of narrative captions}}$) to evaluate performance.

\begin{table}[]
    \centering
    \begin{tabular}{|c|c|c|c|}
    \hline
        Metric & DMR & NMR & Accuracy \\ \hline
        COCO & 0.06 & 0.60 & 0.91 \\ \hline
        CC & 0.15 & 0.64 & 0.69 \\ \hline
        SBUCaps & 0.24 & 0.60 & 0.63 \\ \hline
        RedCaps & 0.53 & 0.32 & 0.60 \\ \hline
    \end{tabular}
    \caption{Using the annotated sets, we evaluate the ability of the descriptiveness classifier to generalize to in-the-wild captions. Except for RedCaps, the part-of-speech based descriptiveness classifier is unable generalize outside of the VIST descriptive/narrative domain. We report misclassification rate for the descriptive captions (DMR) and the narrative captions (NMR), defined in the text.}
    \label{tab:desc_classifier_score_in_wild_annot}
\end{table}

 We show the results in Table \ref{tab:desc_classifier_score_in_wild_annot}. We find that while the descriptiveness classifier is able to correctly identify descriptive captions in most datasets, it struggles with correctly identifying narrative captions. We suspect that this might be due to the domain shift from VIST-SIS to the narratives found in the real world. Furthermore, the features that indicate narrativeness in the natural captions are not represented by part-of-speech features. For example, specific words indicate subjectivety, like ``interesting" and others are concrete ``red", yet both are considered adjectives in terms of part-of-speech. Similarly, first-person pronouns like ``I" and ``my" fall under personal pronouns. But, beyond the part of speech tags, there are implicit first-person perspectives found in the grammatically incorrect short hand writing found in natural captions: ``watching a doggie show in the bar while waiting for the pizza". The underspecification of the features used for the descriptiveness classifier explains why it fails to generalize to narrative captions in-the-wild.
