# Supplementary material for: VEIL: Vetting Extracted Image Labels from In-the-Wild Captions for Weakly-Supervised Object Detection
Source: arXiv:2303.09608 source file (2024-03-10)
Supplement: Supplementary file 3 [file cross_dataset_results.tex]

vspace\begin{table}[!ht]
    \centering
    \begin{tabular}{|l|l|l|l|l|l|l|l|l|l|l|l|l|l|l|l|}
    \hline
        \textbf{Train Dataset} & \textbf{DII-VIST Val} & \textbf{DII-VIST Val} & \textbf{SIS-VIST} & \textbf{SIS-VIST} & \textbf{COCO Val} & \textbf{COCO Val} & \textbf{VIST Val} & \textbf{VIST Val} & \textbf{SBUCaps VAL (41746)} & \textbf{SBUCaps VAL (41746)} & \textbf{RedCaps VAL (211333)} & \textbf{RedCaps VAL (211333)} & \textbf{CC VAL (87510)} & \textbf{CC VAL (87510)} & \textbf{} \\ \hline
        No filtering & 0.779 / 1.000 & 0.876 & 0.695 / 1.000 & 0.820 & 0.948 / 1.000 & 0.973 & 0.741 / 1.000 & 0.851 & 0.463 / 1.000 & 0.633 & 0.596 / 1.000 & 0.747 & 0.737 / 1.000 & 0.849 & ~ \\ \hline
        SBU (166986) & 0.895 / 0.717 & 0.796 & 0.831 / 0.609 & 0.703 & 0.979 / 0.647 & 0.779 & 0.878 / 0.690 & 0.773 & 0.828 / 0.791 & 0.809 & 0.808 / 0.684 & 0.741 & 0.844 / 0.831 & 0.837 & ~ \\ \hline
        RedCaps (813130) & 0.865 / 0.794 & 0.828 & 0.787 / 0.752 & 0.769 & 0.975 / 0.824 & 0.893 & 0.839 / 0.785 & 0.811 & 0.668 / 0.759 & 0.710 & 0.855 / 0.929 & 0.890 & 0.837 / 0.709 & 0.768 & ~ \\ \hline
        CC (350043) & 0.863 / 0.902 & 0.882 & 0.759 / 0.917 & 0.830 & 0.974 / 0.925 & 0.949 & 0.824 / 0.914 & 0.867 & 0.585 / 0.846 & 0.692 & 0.713 / 0.844 & 0.773 & 0.884 / 0.935 & 0.909 & ~ \\ \hline
        VIST & 0.826 / 0.978 & 0.895 & 0.729 / 0.949 & 0.825 & 0.958 / 0.926 & 0.942 & 0.789 / 0.971 & 0.871 & 0.518 / 0.939 & 0.668 & 0.658 / 0.883 & 0.754 & 0.771 / 0.981 & 0.863 & ~ \\ \hline
        COCO & 0.779 / 1.000 & 0.876 & 0.695 / 1.000 & 0.820 & 0.948 / 1.000 & 0.973 & 0.741 / 1.000 & 0.851 & 0.463 / 1.000 & 0.633 & 0.599 / 1.000 & 0.749 & 0.739 / 1.000 & 0.850 & ~ \\ \hline
        SBUCaps+CC & 0.885 / 0.840 & 0.862 & 0.788 / 0.837 & 0.812 & 0.978 / 0.893 & 0.933 & 0.847 / 0.838 & 0.843 & 0.923 / 0.950 & 0.937 & 0.762 / 0.822 & 0.791 & 0.965 / 0.978 & 0.972 & ~ \\ \hline
        RedCaps+CC & 0.876 / 0.888 & 0.882 & 0.801 / 0.784 & 0.793 & 0.976 / 0.918 & 0.946 & 0.855 / 0.852 & 0.854 & 0.691 / 0.720 & 0.705 & 0.845 / 0.836 & 0.841 & 0.892 / 0.914 & 0.903 & ~ \\ \hline
        SBUCaps+Redcaps & 0.876 / 0.779 & 0.825 & 0.789 / 0.697 & 0.741 & 0.976 / 0.791 & 0.874 & 0.849 / 0.758 & 0.801 & 0.892 / 0.940 & 0.915 & 0.923 / 0.958 & 0.940 & 0.846 / 0.785 & 0.810 & ~ \\ \hline
        CC Method w/ special token & 0.868 / 0.913 & 0.890 & 0.765 / 0.920 & 0.836 & 0.975 / 0.942 & 0.958 & 0.835 / 0.920 & 0.875 & 0.609 / 0.841 & 0.707 & 0.721 / 0.862 & 0.785 & 0.922 / 0.955 & 0.938 & ~ \\ \hline
        SBUCaps method w/ special token & 0.885 / 0.798 & 0.839 & 0.817 / 0.719 & 0.765 & 0.977 / 0.745 & 0.846 & 0.866 / 0.768 & 0.814 & 0.790 / 0.814 & 0.802 & 0.782 / 0.754 & 0.767 & 0.834 / 0.866 & 0.850 & ~ \\ \hline
        RedCaps method w/ special token & 0.880 / 0.744 & 0.806 & 0.809 / 0.697 & 0.749 & 0.976 / 0.776 & 0.865 & 0.856 / 0.721 & 0.783 & 0.686 / 0.724 & 0.705 & 0.843 / 0.901 & 0.871 & 0.831 / 0.526 & 0.644 & ~ \\ \hline
        RedCaps+CC w/ special tok & 0.862 / 0.922 & 0.891 & 0.779 / 0.842 & 0.809 & 0.971 / 0.944 & 0.957 & 0.837 / 0.894 & 0.865 & 0.649 / 0.797 & 0.716 & 0.793 / 0.887 & 0.837 & 0.868 / 0.931 & 0.899 & ~ \\ \hline
        SBUCaps+CC w/ special tok & 0.870 / 0.915 & 0.892 & 0.776 / 0.881 & 0.825 & 0.976 / 0.932 & 0.954 & 0.830 / 0.905 & 0.866 & 0.754 / 0.821 & 0.786 & 0.747 / 0.847 & 0.793 & 0.891 / 0.943 & 0.916 & ~ \\ \hline
        SBUCaps+Redcaps w/ special tok & 0.877 / 0.807 & 0.841 & 0.805 / 0.712 & 0.756 & 0.973 / 0.856 & 0.911 & 0.844 / 0.828 & 0.836 & 0.826 / 0.724 & 0.772 & 0.804 / 0.905 & 0.851 & 0.839 / 0.771 & 0.803 & ~ \\ \hline
        SUPER AM & 0.86 / 0.969 & 0.911 & 0.779 / 0.903 & 0.836 & 0.973 / 0.990 & 0.981 & 0.832 / 0.947 & 0.886 & 0.713 / 0.829 & 0.767 & 0.803 / 0.898 & 0.848 & 0.874 / 0.941 & 0.906 & ~ \\ \hline
    \end{tabular}
    \caption{Cross Dataset Vetting Results}
    \label{tab:cross_dataset_all}
\end{table}
